# Supplementary material for: Computational Diplomacy: How "hackathons for good" feed a participatory future for multilateralism in the digital age
Source: arXiv:2410.03286 source file (2024-10-04)
Supplement: Supplementary file 1 [file a_SDGs.tex]

\section{Summary of the 17 UN Sustainable Development Goals (SDGs)}
\label{appendix:SDG}

\begin{enumerate}
    \item \textbf{No Poverty}: Eradicate poverty in all its forms everywhere.
    \item \textbf{Zero Hunger}: End hunger, achieve food security, improve nutrition, and promote sustainable agriculture.
    \item \textbf{Good Health and Well-being}: Ensure healthy lives and promote well-being for all at all ages.
    \item \textbf{Quality Education}: Ensure inclusive and equitable quality education and promote lifelong learning opportunities for all.
    \item \textbf{Gender Equality}: Achieve gender equality and empower all women and girls.
    \item \textbf{Clean Water and Sanitation}: Ensure availability and sustainable management of water and sanitation for all.
    \item \textbf{Affordable and Clean Energy}: Ensure access to affordable, reliable, sustainable, and modern energy for all.
    \item \textbf{Decent Work and Economic Growth}: Promote sustained, inclusive, and sustainable economic growth, full and productive employment, and decent work for all.
    \item \textbf{Industry, Innovation, and Infrastructure}: Build resilient infrastructure, promote inclusive and sustainable industrialisation, and foster innovation.
    \item \textbf{Reduced Inequality}: Reduce inequality within and among countries.
    \item \textbf{Sustainable Cities and Communities}: Make cities and human settlements inclusive, safe, resilient, and sustainable.
    \item \textbf{Responsible Consumption and Production}: Ensure sustainable consumption and production patterns.
    \item \textbf{Climate Action}: Take urgent action to combat climate change and its impacts.
    \item \textbf{Life Below Water}: Conserve and sustainably use the oceans, seas, and marine resources for sustainable development.
    \item \textbf{Life on Land}: Protect, restore, and promote sustainable use of terrestrial ecosystems, manage forests sustainably, combat desertification, and halt biodiversity loss.
    \item \textbf{Peace, Justice, and Strong Institutions}: Promote peaceful and inclusive societies for sustainable development, provide access to justice for all, and build effective, accountable, and inclusive institutions at all levels.
    \item \textbf{Partnerships for the Goals}: Strengthen the means of implementation and revitalise the global partnership for sustainable development.
\end{enumerate}
