# Supplementary material for: Computational Diplomacy: How "hackathons for good" feed a participatory future for multilateralism in the digital age
Source: arXiv:2410.03286 source file (2024-10-04)
Supplement: Supplementary file 2 [file a_data.tex]

\section{Data \& Methods}
\label{appendix:data}

\subsection{Devpost}
\label{sec:devpost}
Devpost is an online platform that connects developers with hackathons, coding contests, and challenges, providing a space to showcase projects, collaborate, and gain recognition. It serves as a hub for innovation and skill development, offering opportunities for both novice and experienced developers to engage in competitive programming and project building.

\subsubsection{Key Features}
Devpost hosts and promotes various hackathons and coding contests, both online and in-person, organized by companies, educational institutions, and communities. This allows developers to work on real-world problems and compete for prizes. Developers can create profiles to showcase their projects with detailed descriptions, images, videos, and links to repositories, building a portfolio of their work. The platform facilitates collaboration by enabling users to form teams and connect with industry professionals, mentors, and potential employers.

Participation in Devpost events helps developers learn new technologies, improve coding skills, and gain hands-on experience. Many events include a judging process where industry experts review and provide feedback on projects, helping developers enhance their skills and gain industry insights. Devpost fosters a supportive community where users can share knowledge, ask for help, and support each other, often featuring resources, webinars, and tutorials.

\subsubsection{How Devpost Works}
Users create an account on Devpost to showcase their skills, projects, and event participation. They can browse and register for upcoming hackathons and challenges, each with specific rules, themes, and submission requirements. During events, participants work on their projects individually or in teams and submit them through Devpost, providing all necessary details and documentation.

Projects are then reviewed by judges based on criteria such as creativity, technical complexity, and impact. Winners are announced and awarded prizes, which can include cash, internships, job offers, or other incentives. Submitted projects are showcased on Devpost, allowing other users to view, comment, and share them, leading to networking opportunities and collaboration offers.

\subsubsection{Example Use Cases}
Universities use Devpost to host hackathons that engage students, foster innovation, and provide practical experience outside the classroom. Companies organize coding contests on Devpost to identify talent, crowdsource solutions, and promote their brand within the developer community. Tech communities and non-profit organizations use Devpost to bring developers together to solve social issues and promote learning and collaboration. Individual developers participate in events to challenge themselves, learn new skills, and build a portfolio of projects to showcase to potential employers.

\subsubsection{Benefits of Using Devpost}
Devpost provides exposure and recognition for developers' work, leading to career opportunities. Participation in diverse challenges enhances skills and facilitates networking with like-minded individuals, mentors, and industry professionals. The competitive nature of hackathons and contests inspires innovation and creative problem-solving. Overall, Devpost plays a crucial role in the tech ecosystem by fostering innovation, skill development, and community engagement among developers.

\subsubsection{Limitations of Devpost}

The empirical work presented in this paper is based on an archival analysis of an existing hackathon platform --- Devpost --- and has, as such, several limitations.
First, the database only covers a small number of hackathons that take place across the globe. Moreover, while Devpost contains information about events that take place all over the globe, most events represented there, took place in Europe or the Americas. The data is thus not representative of all hackathons. This does, however, only pose a minor limitation, since we are not aiming for completeness.
Second, the information presented in Devpost is provided by the organisers and participants of events and might, as such, be incomplete or events can be misrepresented. This is a limitation that we have to accept because it is not possible for us to confirm the information that is provided in Devpost. It can, however, be considered unlikely that organisers would greatly misrepresent their event because Devpost is often used to attract participants who would then consequently be disappointed when attending a hackathon that was described very differently.
Third, we make the conceptual assumption that participants attend a hackathon at least partially because of its theme and focus. This is not necessarily the case, though, because individuals might also participate in hackathons for other reasons, such as joining friends who participate. We argue, though, that individuals will still contribute to a hackathon and thus to the SDGs that it focuses on, even if their original motivation might not have been related.
Fourth, due to the way the data was collected, it only represents one specific point in time. Hackathon descriptions and participant profiles might have changed since we collected them. However, since we focus on hackathons that took place in the past, it can be considered unlikely that organisers would change the description of an event post-hoc.
Fifth, it is common for participants to create GitHub repositories specifically for one event and never use them before or after an event. This does not pose an issue for our analysis, though, since it only leads to us potentially underestimating the activity that takes place before and after an event.

\subsection{GitHub Archive}
\label{sec:github_archive}

\subsubsection{GitHub Archive Overview}
GitHub Archive (\url{https://gharchive.org}) is a project that records the public timeline of events on GitHub, offering a comprehensive, continuously updated archive of GitHub activity. It is designed for researchers, developers, and data analysts to analyze trends, behaviors, and patterns in open-source software development.

\subsubsection{General Data Schema}
GitHub Archive captures a variety of event types, and each event follows a specific schema. The general data schema includes:

\begin{enumerate}
    \item {\bf Event Type:} The type of event, such as `PushEvent`, `PullRequestEvent`, `IssuesEvent`, `WatchEvent`, etc.
    \item {\bf Event ID:} A unique identifier for the event.
    \item {\bf Repository:} Details about the repository where the event occurred, including: `id`: Repository ID, `name`: Full name of the repository (`owner/repo`), `url`: URL to the repository.
    \item {\bf Actor:} Information about the user who triggered the event, including: `id`: User ID, `login`: Username, `url`: URL to the user’s GitHub profile.
    \item {\bf Organization (optional):} Information about the organization related to the event, if applicable.
    \item {\bf Payload:} The payload varies depending on the event type and includes detailed information about the event, such as: `PushEvent`: List of commits, commit messages, commit IDs, etc.; `PullRequestEvent`: Pull request details, state, merged status, etc.; For `IssuesEvent`: Issue details, state, comments, etc.
    \item {\bf Public:} A boolean indicating if the event is public.
    \item {\bf Created At:} The timestamp when the event was created.
\end{enumerate}

\subsubsection{Time Ranges and Resolutions}

\begin{itemize}
    \item {\bf Historical Data:} GitHub Archive provides data starting from February 12, 2011.
    \item {\bf Real-time Updates:} Data is continuously updated, capturing real-time GitHub activity.
\end{itemize}

Resolutions: The data is divided into hourly archives. Each hour's data is stored in a JSON file that can be accessed via HTTP or downloaded for local analysis. It can also be downloaded in aggregated monthly or yearly tables.

\subsubsection{Data Accessibility}

\begin{enumerate}
    \item {\bf HTTP Access:} Users can access the hourly JSON files directly via HTTP, enabling them to download specific time periods of data.
    \item {\bf Google BigQuery:} For advanced querying and analysis, the dataset is integrated with Google BigQuery. This allows users to run complex SQL queries on the data without needing to download and store large volumes of JSON files locally.

\end{enumerate}

Example JSON Structure for an Event:
\begin{Verbatim}[breaklines=true]
    {
  "id": "1234567890",
  "type": "PushEvent",
  "actor": {
	"id": 123456,
	"login": "username",
	"display_login": "username",
	"gravatar_id": "",
	"url": "https://api.github.com/ users/
 username",
	"avatar_url": "https:// avatars.githubusercontent.com/ u/123456?"
  },
  "repo": {
	"id": 12345678,
	"name": "owner/repo",
	"url": "https://api.github.com/repos/owner/ repo"
  },
  "payload": {
	"push_id": 1234567890,
	"size": 1,
	"distinct_size": 1,
	"ref": "refs/heads/main",
	"head": "abc123def456",
	"before": "abc123def455",
	"commits": [
  	{
    	"sha": "abc123def456",
    	"author": {
      	"email": "author@example.com",
      	"name": "Author Name"
    	},
    	"message": "Commit message",
    	"distinct": true,
    	"url": "https://api.github.com/repos/ owner/repo/commits/abc123def456"
  	}
	]
  },
  "public": true,
  "created_at": "2024-05-16T12:34:56Z"
}
\end{Verbatim}

GitHub Archive provides a valuable resource for analysing the dynamics of GitHub's open-source ecosystem, offering detailed and structured data for a wide range of applications.
