# Supplementary material for: Computational Diplomacy: How "hackathons for good" feed a participatory future for multilateralism in the digital age
Source: arXiv:2410.03286 source file (2024-10-04)
Supplement: Supplementary file 3 [file a_summit_of_future.tex]

\subsection{Multilateralism and The Summit of the Future}
\label{appendix:summit_of_the_future}

\subsubsection{Origins of Multilateralism}
Multilateralism traces its origins to the early twentieth Century, emerging prominently after World War I with the founding of the League of Nations in 1920. This concept was developed to foster international cooperation and prevent conflicts, recognising that many world issues transcend national borders and necessitate collective action. The establishment of the United Nations (UN) after World War II marked a significant advancement in multilateralism, setting a framework for global diplomacy and international law, guided by principles such as sovereign equality and peaceful dispute resolution between nation states.

International organisations under the multilateral framework, such as the United Nations, the World Bank, and the World Health Organisation, aim to address a variety of global issues, including peace and security, economic development, and health crises. Their missions involve promoting human rights, facilitating economic development, mitigating conflicts, and providing humanitarian aid in crises.

However, the efficacy of these organisations is increasingly challenged by a changing world. Current shortcomings include issues like bureaucracy and slow decision-making processes, lack of enforcement mechanisms, disparities in the influence and contribution of member states, and occasionally, a failure to adapt to new global dynamics such as digitisation and climate change. These gaps have sparked debates on the need for reforms to better align with the fast-evolving global landscape, ensuring that multilateralism remains an effective tool for international collaboration in the 21st century.

\subsubsection{The Summit of the Future}
Recognizing the urgency of reforming itself, the United Nations have called to hold the Summit of the Future. This conference, to be held in September 2024, is deemed as a one-of-a-kind moment aiming to redefine and strengthen multilateralism for a better future. Following the recommendations of the High-Level Advisory Board on Effective Multilateralism (HLAB), the Summit of the Future has been designed to reassert the commitments to key international goals such as the Sustainable Development Goals (SDGs), the UN Charter, and to promote a rejuvenated, more effective multilateral system that can positively impact people's lives worldwide. The backdrop to this summit includes recent global crises such as the climate emergency, the COVID-19 pandemic, the war in Ukraine, and exponentially paced technological changes disrupting the socioeconomic landscape. These extreme events along with many, however not less disruptive, local events, have tested the resilience and efficacy of international institutions, which have been primarily designed to support multilateralism and to alleviate human and social disasters. Emphasising the urgent need for unified action based on shared principles and objectives, UN Secretary-General António Guterres highlighted the summit as a unique chance to rebuild trust and align outdated multilateral frameworks with today's global landscape, characterised by equity and solidarity. It aims to mitigate risks and foster a safer, more peaceful world. The Summit of the Future is organised around 6 shifts: 
Rebuild Trust in Multilateralism: Improve legitimacy and effectiveness through inclusion and accountability
Planet and People: Regain balance with nature and provide clean energy for all
Global Finance: Ensure sustainable finance that delivers for all	
Digital and Data Governance: Support a just digital transition that unlocks the value of data and protects against digital harms							
Peace and Prevention: Empower effective, equitable collective security arrangements
Anticipatory Action: Strengthen governance for current and emerging transnational risks

At its core, the Summit of the Future is driven by the vision laid out in the Secretary-General's 2021 report, ``Our Common Agenda," which advocates for an inclusive, networked, and efficient form of multilateralism. This initiative seeks to accelerate progress towards the 17 SDGs, with a concerted effort to overcome setbacks caused by the pandemic and other global challenges. A key outcome expected from the summit is the adoption of the Pact for the Future, encompassing five critical areas: sustainable development and financing, international peace and security, science, technology, innovation and digital cooperation, youth and future generations, and transforming global governance. This pact is seen as a commitment among nations to leverage global tools to address emergent issues proactively .
One of the six shifts emphasized in the preparatory discussions for the Summit involves new forms of people engagement and collective intelligence, crucial for rebuilding trust in multilateralism. This shift acknowledges the imperative of involving a broader spectrum of society in decision-making processes, particularly the youth. With over half of the world's population under 30, the summit emphasizes the need for young people to have a meaningful seat at the decision-making table. This approach is not just about consulting young people but involves recognizing them as true and equal partners in crafting a sustainable future.
The discussions and policy briefs leading up to the Summit have underscored the need for a more networked, inclusive, and effective UN system to accelerate SDG implementation. This entails fostering enablers of SDG acceleration, such as digitalization and access to finance, addressing obstacles to SDG realization, reinforcing international standards supportive of SDGs, and enhancing UN development cooperation and financing. The overarching goal is to bridge the significant gap between global challenges and the UN's capacity to respond effectively, thereby strengthening international cooperation and trust, especially among developing nations.
In essence, the Summit of the Future aims to catalyze a global movement towards more effective, inclusive, and networked multilateralism. By embracing new forms of engagement and leveraging collective intelligence, the summit seeks to establish a more resilient, equitable, and sustainable framework for addressing the complex challenges of today and tomorrow.
